# Supplementary material for: Enabling Team of Teams: A Trust Inference and Propagation (TIP) Model in Multi-Human Multi-Robot Teams
Source: arXiv:2305.12614 source file (2024-07-15)
Supplement: Supplementary file 1 [file appendix_v1.tex]

\section*{Appendix}


\subsection{Proof of Theorem \ref{thm:both_converge}}
% We separate the cases into $n=0$ and $n >0$.
\noindent\textbf{Case 1}: $n=0$. We prove in three steps.

First, we show that $t_{k}^{x,A}$ converges i.p.. When $n=0$, $x$ gains experience towards $A$ through only direct interaction, and thus, by Eq.~\eqref{eq:direct_update},
\begin{equation}
\label{eq:direct_only_limit}
\begin{aligned}
 & \lim _{k\rightarrow \infty }\frac{\alpha _{k}^{x,A}}{\alpha _{k}^{x,A} +\beta _{k}^{x,A}}\\
= & \lim _{k\rightarrow \infty }\frac{\alpha _{0}^{x,A} +ks^{x,A} r}{\alpha _{0}^{x,A} +\beta _{0}^{x,A} +kf^{x,A}\overline{r} +ks^{x,A} r}\\
= & \frac{s^{x,A} r}{f^{x,A}\overline{r} +s^{x,A} r} .
\end{aligned}
\end{equation}
For any $\epsilon  >0$, by the Markov inequality, 
\begin{equation}
\label{eq:markov}
\begin{aligned}
 & \lim _{k\rightarrow \infty }\Pr\left(\left| t_{k}^{x,A} -\mu _{k}^{x,A}\right| < \epsilon \right)\\
\leqslant  & \lim _{k\rightarrow \infty }\frac{1}{\epsilon ^{2}}\mathbb{E}\left[\left( t_{k}^{x,A} -\mu _{k}^{x,A}\right)^{2}\right] =0,
\end{aligned}
\end{equation}
where the last equality is true because $\lim _{k\rightarrow \infty }\operatorname{Var}\left( t_{k}^{x,A}\right) =0$ as $\lim _{k\rightarrow \infty }\left( \alpha _{k}^{x,A} +\beta _{k}^{x,A}\right) =\infty $. Let $t^{x} =\frac{s^{x,A} r}{f^{x,A}\overline{r} +s^{x,A} r}$. Eq.'s \eqref{eq:direct_only_limit} and \eqref{eq:markov} yields 
\begin{equation}
\lim _{k\rightarrow \infty }\Pr\left(\left| t_{k}^{x,A} -t^{x}\right| < \epsilon \right) =1.
\end{equation}

Second, we show $\left| \mu _{k-1}^{y,A} -t_{k}^{x,A}\right| $ converge i.p. to zero. Suppose this is not true. We consider the following equation:
\begin{equation}
\label{eq:mu_limit_1}
\begin{aligned}
 & \left| \mu _{k+m-1}^{y,A} -t_{k+m}^{x,A}\right| \\
= & \left| \mu _{k-1}^{y,A} -t_{k}^{x,A}\right| \prod _{j=1}^{m}\frac{\left| \mu _{k+j-1}^{y,A} -t_{k+j}^{x,A}\right| }{\left| \mu _{k+j-2}^{y,A} -t_{k+j-1}^{x,A}\right| }
\end{aligned} .
\end{equation}
As we have shown $t_{k}^{x,A}\xrightarrow{\text{i.p.}} t^{x}$ when $k\rightarrow \infty $, by the continuous mapping theorem, when $k\rightarrow \infty $, 
\begin{equation}
\label{eq:mu_limit_2}
\begin{aligned}
 & \left| \mu _{k-1}^{y,A} -t_{k}^{x,A}\right| \prod _{j=1}^{m}\frac{\left| \mu _{k+j-1}^{y,A} -t_{k+j}^{x,A}\right| }{\left| \mu _{k+j-2}^{y,A} -t_{k+j-1}^{x,A}\right| }\\
\xrightarrow{\text{i.p.}} & \left| \mu _{k-1}^{y,A} -t^{x}\right| \prod _{j=1}^{m}\frac{\left| \mu _{k+j-1}^{y,A} -t^{x}\right| }{\left| \mu _{k+j-2}^{y,A} -t^{x}\right| } .
\end{aligned}
\end{equation}
As we assume $\mu _{k-1}^{y,A}\xrightarrow{\text{i.p.}} t_{k}^{x,A}$, there exist $\epsilon ,\ \delta  >0$ such that there are infinite many $k$'s such that $\Pr\left(\left| \mu _{k-1}^{y,A} -t_{k}^{x,A}\right|  >\epsilon \right)  >\delta $. As a result, by Eq.'s \eqref{eq:indirect_update} and \eqref{eq:trust_expected},
\begin{equation}
\label{eq:mu_limit_3}
\prod _{j=1}^{m}\frac{\left| \mu _{k+j-1}^{y,A} -t^{x}\right| }{\left| \mu _{k+j-2}^{y,A} -t^{x}\right| }\xrightarrow{\text{i.p.}} 0
\end{equation}
when $m\rightarrow \infty $. Eq.'s \eqref{eq:mu_limit_1}, \eqref{eq:mu_limit_2}, and \eqref{eq:mu_limit_3} together yield $\left| \mu _{k+m-1}^{y,A} -t_{k+m}^{x,A}\right| \xrightarrow{\text{i.p.}} 0$ when both $k$ and $m$ tend to infinity, which contradicts our assumption. Therefore, $\left| \mu _{k-1}^{y,A} -t_{k}^{x,A}\right| \xrightarrow{\text{i.p.}} 0$. In addition, $\mu _{k}^{y,A}\xrightarrow{\text{i.p.}} t^{x}$ since $t_{k}^{x,A}\xrightarrow{\text{i.p.}} t^{x}$.

Third, we show $\left| \mu _{k}^{y,A} -t_{k}^{y,A}\right| \xrightarrow{\text{i.p.}} 0$. Suppose this is not true. Then we have $\alpha _{k}^{y,A} +\beta _{A}^{y,A} < \infty $; otherwise, similar to Eq. \eqref{eq:markov}, we can show $\left| \mu _{k}^{y,A} -t_{k}^{y,A}\right| \xrightarrow{\text{i.p.}} 0$. However, $\alpha _{k}^{y,A} +\beta _{A}^{y,A} < \infty $ will imply $\mu _{k}^{y,A}$ cannot converge to a constant i.p. due to the indirect trust update rule in Eq.~\eqref{eq:indirect_update}, which is a contradiciton. Thus, we have $\left| \mu _{k}^{y,A} -t_{k}^{y,A}\right| \xrightarrow{\text{i.p.}} 0$.

Therefore, both $t_{k}^{x,A}$ and $t_{k}^{y,A}$ converge to $t^{x}$ i.p..

\vspace{2mm}
\noindent\textbf{Case 2}: $n >0$.

First, when $k\rightarrow \infty $, $\alpha _{k}^{x,A}$, $\beta _{k}^{x,A}$, $\alpha _{k}^{y,A}$, and $\beta _{k}^{y,A}$ all go to infinity as both $x$ and $y$ will have an infinite number of direct interactions with $A$. As a result, we have
\begin{equation}
\label{eq:t_deviation_go_to_zero}
\begin{aligned}
\left| t_{k}^{x,A} -\mu _{k}^{x,A}\right|  & \xrightarrow{\text{i.p.}} 0 & \text{and}\\
\left| t_{k}^{y,A} -\mu _{k}^{y,A}\right|  & \xrightarrow{\text{i.p.}} 0. & 
\end{aligned}
\end{equation}

Second, we show $\Delta t_{k} :=t_{k}^{x,A} -t_{k}^{y,A}$ converges to some constant. It can be shown that $\Delta t_{k}$ is Cauchy in probability and thus converges to some random variable $\Delta t^{'}$. As 
\begin{equation}
\begin{aligned}
 & | \Delta t_{k} -\mathbb{E}[ \Delta t_{k}]| \\
= & \left| \left( t_{k}^{x,A} -\mu _{k}^{x,A}\right) -\left( t_{k}^{y,A} -\mu _{k}^{y,A}\right)\right| 
\end{aligned}
\end{equation}
and its right-hand side converges to zero i.p., $| \Delta t_{k} -\mathbb{E}[ \Delta t_{k}]| $ also converges to zero i.p, which implies $\operatorname{Var}\left( \Delta t^{'}\right) =0$. Therefore,
\begin{equation}
\label{eq:t_detivation_goto_0_2}
t_{k}^{x,A} -t_{k}^{y,A}\xrightarrow{\text{i.p.}} \Delta t,
\end{equation}
where $\Delta t$ is a constant. 

Finally, we show $t_{k}^{x,A}$ and $t_{k}^{y,A}$ converge to constants i.p.. Since $\left| \mu _{k}^{x,A} -\mu _{k-1}^{x,A}\right| \xrightarrow{\text{i.p.}} 0$, by \eqref{eq:t_deviation_go_to_zero} and \eqref{eq:t_detivation_goto_0_2}, we obtain
\begin{equation}
\left| t_{k}^{y,A} -\mu _{k-1}^{x,A}\right| \xrightarrow{\text{i.p.}} \Delta t.
\end{equation}
By \eqref{eq:indirect_update} and \eqref{eq:direct_update}, both indirect and direct experience gains of $y$ converge to some constants i.p. Therefore, the ratio $\frac{\ \alpha _{k}^{y,A}}{\alpha _{k}^{y,A} +\beta _{k}^{y,A}}$ converge to some constants i.p. respectively, i.e., there exist some $t^{y}$ such that $t_{k}^{y,A}\xrightarrow{\text{i.p.}} t^{y}$. Similarly, there exists some $t^{x}$ such that $t_{k}^{x,A}\xrightarrow{\text{i.p.}} t^{x}$.

\qed 
\subsection{Proof of Theorem \ref{thm:equilibria}}
When $n=0$, \eqref{eq:equilibria_case1} yields $t^{x} =t^{y} =\frac{s^{x,A} r}{f^{x,A}\overline{r} +s^{x,A} r}$, which agrees the proof of theorem \ref{thm:both_converge}.

Now we consider the case $n >0$. Let $t^{x}$ and $t^{y}$ be the equilibria in the statement. If $S^{x} /F^{x} -S^{y} /F^{y} \geqslant 0$, it can be shown that
\begin{equation*}
\lim\limits _{k\rightarrow \infty }\Pr\left( t_{k}^{x,A} -t_{k}^{y,A} \geqslant 0\right) =1.
\end{equation*}
As a result, we have
\begin{equation}
\label{eq:trust_delta}
\begin{aligned}
\left[ \mu _{k-1}^{y,A} -t_{k}^{x,A}\right]^{+} & \xrightarrow{\text{i.p.}} 0 & \text{ and }\\
\ \ \left[ t_{k}^{x,A} -\mu _{k-1}^{y,A}\right]^{+} & \xrightarrow{\text{i.p.}} t^{x} -t^{y} . & 
\end{aligned}
\end{equation}
When $k\rightarrow \infty $, by \eqref{eq:direct_update}, \eqref{eq:indirect_update}, and \eqref{eq:trust_delta}, we have 
\begin{equation}
\begin{aligned}
\alpha _{kl+l}^{x,A} -\alpha _{kl}^{x,A} & \xrightarrow{\text{i.p.}} S_{A}^{x}\\
\beta _{kl+l}^{x,A} -\beta _{kl}^{x,A} & \xrightarrow{\text{i.p.}}\hat{F}_{A}^{x}\left( t^{x} -t^{y}\right) +F_{A}^{x}
\end{aligned} ,
\end{equation}
where $l=m+n$. This implies the trust gains are constant every other $l$ interactions. By \eqref{eq:trust_def},
\begin{equation}
\begin{aligned}
t^{x} & =\lim _{k\rightarrow \infty }\frac{\ \alpha _{k}^{x,A}}{\alpha _{k}^{x,A} +\beta _{k}^{x,A}}\\
 & =\frac{S_{A}^{x}}{S_{A}^{x} +\hat{F}_{A}^{x}\left( t^{x} -t^{y}\right) +F_{A}^{x}} ,
\end{aligned}
\end{equation}
which prove the first equation in \eqref{eq:equilibria_case1}. The second equation in \eqref{eq:equilibria_case1} can be proved similarly.

The proof for the case when $S_{A}^{x} /F_{A}^{x} -S_{A}^{y} /F_{A}^{y} < 0$ is similar.

\qed 


\subsection{Proof of Theorem \ref{thm:bound_inference_optimum}}
First of all,
\begin{equation}
\label{eq:H_H_diff_1}
\begin{aligned}
 & \left| \tilde{H}\left(\tilde{\theta }^{*}\right) -H\left( \theta ^{*}\right)\right| \\
\leqslant  & \max\left\{\tilde{H}\left(\tilde{\theta }^{*}\right) -H\left(\tilde{\theta }^{*}\right) ,H\left( \theta ^{*}\right) -\tilde{H}\left( \theta ^{*}\right)\right\}\\
\leqslant  & \max\left| \tilde{H}( \theta ) -H( \theta )\right| 
\end{aligned}
\end{equation}
The log PDF of a Beta random variable $t\sim \operatorname{Beta}( \alpha ,\beta )$ is 
\begin{equation}
\label{eq:log_beta_PDF}
\begin{aligned}
 & \log\operatorname{Beta}( t;\alpha ,\beta )\\
= & -\log\operatorname{B}( \alpha ,\beta ) +( \alpha -1)\log t+( \beta -1)\log( 1-t) ,
\end{aligned}
\end{equation}
By \eqref{eq:likelihood_def}, \eqref{eq:likelihood_app_def}, \eqref{eq:H_H_diff_1}, and \eqref{eq:log_beta_PDF}, we obtain

\begin{equation}
\label{eq:H_H_diff_2}
\begin{aligned}
 & \left| \tilde{H}\left(\tilde{\theta }^{*}\right) -H\left( \theta ^{*}\right)\right| \\
\leqslant  & \max_{\theta }\left\{\sum _{k=0}^{K}\left| \log\operatorname{B}( \alpha _{k} ,\beta _{k}) -\log\operatorname{B}\left(\tilde{\alpha }_{k} ,\tilde{\beta }_{k}\right)\right| +\right. \\
 & \left. \left| \sum _{k=0}^{K}\left[\left(\tilde{\alpha }_{k} -\alpha _{k}\right)\log t_{k} +\left(\tilde{\beta }_{k} -\beta _{k}\right)\log( 1-t_{k})\right]\right| \right\} ,
\end{aligned}
\end{equation}
where $\alpha _{k} ,\beta _{k} ,\tilde{\alpha }_{k} ,\tilde{\beta }_{k}$ are computed according to \eqref{eq:alpha_k_beta_k} and \eqref{eq:alpha_k_beta_k_app}. Here, for the sake of readability, we omit the subscripts. We can bound the second term of the RHS of \eqref{eq:H_H_diff_2} by
\begin{equation}
\begin{aligned}
 & \left| \sum _{k=0}^{K}\left[\left(\tilde{\alpha }_{k} -\alpha _{k}\right)\log t_{k} +\left(\tilde{\beta }_{k} -\beta _{k}\right)\log( 1-t_{k})\right]\right| \\
\leqslant  & T_{K}\left(\sum _{k=0}^{K}\Vert \Delta \mathbf{x}_{k}\Vert _{2}^{2}\right)^{1/2} ,
\end{aligned}
\end{equation}
where $T_{K} =\left(\sum _{k=0}^{K}\left[\log t{_{k}}^{2} +\log( 1-t_{k})^{2}\right]\right)^{1/2}$. The remaining work is to bound the differences of log Beta terms in \eqref{eq:H_H_diff_2}. We complete this in two major steps, namely, approximating the log Beta function and bounding the deviation $\sum _{k=0}^{K}\Vert \Delta \mathbf{x}_{k}\Vert _{2}^{2}$.

\subsubsection{Approximating log Beta Function}
\begin{lemma}
\label{lm:logBeta_approx}
Let $\operatorname{B}$ be the Beta function. Define following functions on $[ 1,\infty )^{2}$:
\begin{equation}
\begin{aligned}
Q( a,b) = & \left( a-\frac{1}{2}\right)\log a+\left( b-\frac{1}{2}\right)\log b\\
 & -\left( a+b-\frac{1}{2}\right)\log( a+b) +\frac{1}{2}\log 2\pi \\
R( a,b) = & \int _{0}^{\infty} \left[\frac{2\arctan\left(\frac{t}{a}\right)}{e^{2\pi t} -1} +\frac{2\arctan\left(\frac{t}{b}\right)}{e^{2\pi t} -1}\right. \\
 &  \left. -\frac{2\arctan\left(\frac{t}{a+b}\right)}{e^{2\pi t} -1}\right] \ \mathrm{d} t\\
\tilde{R}( a,b) = & {\displaystyle \frac{1}{12}\left(\frac{1}{a} +\frac{1}{b} -\frac{1}{a+b}\right)}\\
R_{\delta }( a,b) = & {\displaystyle \frac{1}{30}\left(\frac{1}{a} +\frac{1}{b} -\frac{1}{a+b}\right)}
\end{aligned}
\end{equation}
Then
\begin{equation}
\label{eq:logBeta_Q_R}
\log\operatorname{B}( a,b) =Q( a,b) +R( a,b) ,
\end{equation}
where the residual $R( a,b)$ is positive and approximated by $\tilde{R}( a,b)$. The difference satisfies
\begin{equation}
0< \tilde{R}( a,b) -R( a,b) < R_{\delta }( a,b) .
\end{equation}
\end{lemma}
\begin{proof}

The Beta function can be expressed as
\begin{equation}
\label{eq:log_beta_expression}
{\displaystyle \mathrm{B} (a,b)=\frac{\Gamma ( a+b)}{\Gamma ( a) \Gamma ( b)} ,}
\end{equation}
where $\Gamma $ is the Gamma function. Applying the Binet’s second expression for $\log \Gamma $ (page 260, \cite{whittaker_watson_2021}) to \eqref{eq:log_beta_expression}, we obtain \eqref{eq:logBeta_Q_R}.

It's easy to show, for any $t\geqslant 0,$ and $a,b >1$,
\begin{equation}
\begin{aligned}
 & {\displaystyle \frac{1}{\pi e^{2\pi t}}\left(\frac{1}{a} +\frac{1}{b} -\frac{1}{a+b}\right)}\\
\leqslant  & {\displaystyle \frac{2}{e^{2\pi t} -1}\left(\arctan\left(\frac{t}{a}\right) +\arctan\left(\frac{t}{b}\right)\right. }\\
 & {\displaystyle \left. -\arctan\left(\frac{t}{a+b}\right)\right)}\\
\leqslant  & {\displaystyle \frac{2t}{{\displaystyle e^{2\pi t} -1}}\left(\frac{1}{a} +\frac{1}{b} -\frac{1}{a+b}\right) .}
\end{aligned}
\end{equation}
Integrating each line above on $[ 0,\infty )$ yields
\begin{equation}
{\displaystyle \frac{1}{2\pi ^{2}}\left(\frac{1}{a} +\frac{1}{b} -\frac{1}{a+b}\right)} \leqslant R( a,b) \leqslant {\displaystyle \tilde{R}( a,b) ,}
\end{equation}
which also implies 
\begin{equation}
\begin{aligned}
 & {\displaystyle \tilde{R}( a,b) -} R( a,b)\\
\leqslant  & {\displaystyle \tilde{R}( a,b) -\frac{1}{2\pi ^{2}}\left(\frac{1}{a} +\frac{1}{b} -\frac{1}{a+b}\right)}\\
\leqslant  & R_{\delta }( a,b) .
\end{aligned}
\end{equation}
\end{proof}

For any $a_{1} ,b_{1} ,a_{2} ,b_{2} \geqslant 1$, let $\mathbf{x}_{1} =( a_{1} ,b_{1})$, $\mathbf{x_{2}} =( a_{2} ,b_{2})$ and $\Delta \mathbf{x} =( \Delta a,\Delta b) :=\mathbf{x_{2}} -\mathbf{x_{1}}$. By Lemma~\ref{lm:logBeta_approx}, 
\begin{equation}
\label{eq:logBeta_bound_1}
\begin{aligned}
 & | \log\operatorname{B}(\mathbf{x}_{1}) -\log\operatorname{B}(\mathbf{x}_{2})| \\
\leqslant  & | Q(\mathbf{x}_{1}) -Q(\mathbf{x}_{2})| +| R(\mathbf{x}_{1}) -R(\mathbf{x}_{2})| \\
\leqslant  & | Q(\mathbf{x}_{1}) -Q(\mathbf{x}_{2})| +| \tilde{R}(\mathbf{x}_{1})| +|\tilde{R}(\mathbf{x}_{2})| 
\end{aligned}
\end{equation}
The first order Taylor expansion of $Q$ gives
% term on the RHS of \eqref{eq:logBeta_bound_1} satisfies
\begin{equation}
\label{eq:Q_bound_1}
\begin{aligned}
 & | Q(\mathbf{x}_{2}) -Q(\mathbf{x}_{1})| \\
= & | \nabla Q(\mathbf{x}_{1}) \cdot \Delta \mathbf{x} +\frac{1}{2} \Delta \mathbf{x}^{T}\operatorname{H}_{Q}(\mathbf{x}) \Delta \mathbf{x}| \\
\leqslant  & | \nabla Q(\mathbf{x}_{1}) \cdot \Delta \mathbf{x}| +\frac{1}{2}\left| \Delta \mathbf{x}^{T}\operatorname{H}_{Q}(\mathbf{x}) \Delta \mathbf{x}\right| \\
= & | \nabla Q(\mathbf{x}_{1}) \cdot \Delta \mathbf{x}| +\frac{1}{2} \Delta \mathbf{x}^{T}\operatorname{H}_{Q}(\mathbf{x}) \Delta \mathbf{x} ,
\end{aligned}
\end{equation}
where $\mathbf{x} =( a,b) :=\mathbf{x}_{1} +c\mathbf{h}$, for some $c\in [ 0,1]$, and the last equality is true because the Hessian matrix $\operatorname{H}_{Q}$ of $Q$ is positive definite. \eqref{eq:logBeta_bound_1} and \eqref{eq:Q_bound_1} give the following corollary.
\begin{corollary}
For any $\mathbf{x}_{1} ,\mathbf{x}_{2} \in \ [ 1,\infty )^{2}$, 
\begin{equation}
\label{eq:logB_diff_bound_initial}
\begin{aligned}
 & | \log\operatorname{B}(\mathbf{x}_{1}) -\log\operatorname{B}(\mathbf{x}_{2})| \\
\leqslant  & | \nabla Q(\mathbf{x}_{1}) \cdot \Delta \mathbf{x}| +\frac{1}{2} \Delta \mathbf{x}^{T}\operatorname{H}_{Q}(\mathbf{x}) \Delta \mathbf{x}\\
 & +| \tilde{R}(\mathbf{x}_{1})| +| \tilde{R}(\mathbf{x}_{2})| ,
\end{aligned}
\end{equation}
for some $\mathbf{x}:=\mathbf{x}_{1} +c\mathbf{h}$, $c\in [ 0,1]$.
\end{corollary}

Next, we express \eqref{eq:logB_diff_bound_initial} in elementary functions of $\mathbf{x}_{1}$ and $\mathbf{x}_{2}$. Calculation shows
\begin{equation}
\label{eq:nabla_Q_bound}
\begin{aligned}
 & | \nabla Q(\mathbf{x}_{1}) \cdot \Delta \mathbf{x}| \\
= & \left[\log\left( 1+b_{1} a_{1}^{-1}\right)| \Delta a| +\log\left( 1+a_{1} b_{1}^{-1}\right)| \Delta b| \right]\\
 & +\frac{1}{2}( a_{1} +b_{1})^{-1}\left[ b_{1} a_{1}^{-1}| \Delta a| +a_{1} b_{1}^{-1}| \Delta b| \right]\\
\leqslant  & \sqrt{\log^{2}\left( 1+b_{1} a_{1}^{-1}\right) +\log^{2}\left( 1+a_{1} b_{1}^{-1}\right)}\Vert \Delta \mathbf{x}\Vert \\
 & +\frac{1}{2}( a_{1} +b_{1})^{-1}\sqrt{b_{1}^{2} a_{1}^{-2} +a_{1}^{2} b_{1}^{-2}}\Vert \Delta \mathbf{x}\Vert \\
\leqslant  & \xi (\mathbf{x}_{1})\Vert \Delta \mathbf{x}\Vert ,
\end{aligned}
\end{equation}
where the first inequality comes from the Hölder's inequality, the second inequality comes from the inequality that $\log^{2}( 1+x) < \frac{2}{3} x$ for $x >0$, and
\begin{equation*}
\xi (\mathbf{x}_{1}) =\sqrt{\frac{2}{3}\left(\frac{b_{1}}{a_{1}} +\frac{a_{1}}{b_{1}}\right)} +\frac{1}{2( a_{1} +b_{1})}\sqrt{\frac{b_{1}^{2}}{a_{1}^{2}} +\frac{a_{1}^{2}}{b_{1}^{2}}};
\end{equation*}
and
\begin{equation}
\label{eq:H_Q_bound}
\begin{aligned}
 & \Delta \mathbf{x}^{T}\operatorname{H}_{Q}(\mathbf{x}) \Delta \mathbf{x}\\
= & \rho ( a) \Delta a^{2} +\rho ( b) \Delta b^{2} -\rho ( a+b)( \Delta a+\Delta b)^{2}\\
\leqslant  & \rho ( a) \Delta a^{2} +\rho ( b) \Delta b^{2}\\
\leqslant  & \max\{\rho ( a) ,\rho ( b)\}\Vert \Delta \mathbf{x}\Vert _{2}^{2}\\
\leqslant  & 2\kappa (\mathbf{x}_{1} ,\mathbf{x}_{2})\Vert \Delta \mathbf{x}\Vert _{2}^{2},
\end{aligned}
\end{equation}
where $\rho ( x) =x^{-1} +\frac{1}{2} x^{-2}$ for $x\in [ 1,\infty )$ and $\kappa (\mathbf{x}_{1} ,\mathbf{x}_{2}) =\frac{1}{2}\max\{\rho ( a_{1}) ,\rho ( a_{2}) ,\rho ( b_{1}) ,\rho ( b_{2})\}$.

Substituting \eqref{eq:nabla_Q_bound} and \eqref{eq:H_Q_bound} to \eqref{eq:logB_diff_bound_initial}, we obtain
\begin{equation}
\label{eq:logB_diff_bound}
\begin{aligned}
 & |\log\operatorname{B}(\mathbf{x}_{1}) -\log\operatorname{B}(\mathbf{x}_{2}) |\\
\leqslant  & \xi (\mathbf{x}_{1})\Vert \Delta \mathbf{x}\Vert + \kappa (\mathbf{x}_{1} ,\mathbf{x}_{2})\Vert \Delta \mathbf{x}\Vert _{2}^{2}\\
 & +|\tilde{R}(\mathbf{x}_{1}) |+|\tilde{R}(\mathbf{x}_{2}) |.
\end{aligned}
\end{equation}

\subsubsection{Bound Deviation}
First, we introduce the following lemma for later use.
\begin{lemma}
\label{lmm:inequality_abc}
For any $x_{i} ,y_{i} ,a_{i} ,b_{i} ,c_{i} ,h_{i} \in \mathbb{R}$, $a_{i} ,b_{i} ,c_{i} ,h_{i} \geqslant 0$, such that $h_{i} =\max\{a_{i} ,b_{i}\}$, $| x_{i} -y_{i}| \leqslant c_{i}$ and $| x_{i} +y_{i}| \leqslant c_{i}$, $\forall i\in I_{k}$, where $I_{k}$'s are index sets and satisfy$I_{1} \subset \dotsc \subset I_{K}$, we have 
\begin{equation}
\sum _{k=1}^{K}\bigl[\bigl(\sum _{i\in I_{k}} a_{i} x_{i}\bigr)^{2} +\bigl(\sum _{i\in I_{k}} b_{i} y_{i}\bigr)^{2}\bigr] \leqslant \bigl(\sum _{j=1}^{K}\sum _{i\in I_{j}} h_{i}^{2}\bigr)\bigl(\sum _{k\in I_{K}} c_{k}^{2}\bigr)
\end{equation}
\end{lemma}
\begin{proof}
First, we have
\begin{equation*}
\begin{aligned}
 & (\sum _{i\in I_{k}} a_{i} x_{i})^{2} +(\sum _{i\in I_{k}} b_{i} y_{i})^{2} \leqslant (\sum _{i\in I_{k}} a_{i}| x_{i}| )^{2} +(\sum _{i\in I_{k}} b_{i}| y_{i}| )^{2}\\
\leqslant  & (\sum _{i\in I_{k}} h_{i}| x_{i}| )^{2} +(\sum _{i\in I_{k}} h_{i}| y_{i}| )^{2}\\
\leqslant  & (\sum _{i\in I_{k}} h_{i}^{2})(\sum _{i\in I_{k}} x{_{i}}^{2}) +(\sum _{i\in I_{k}} h_{i}^{2})(\sum _{i\in I_{k}} y{_{i}}^{2})\\
= & (\sum _{i\in I_{k}} h_{i}^{2})(\sum _{i\in I_{k}}( x{_{i}}^{2} +y{_{i}}^{2})) \leqslant (\sum _{i\in I_{k}} h_{i}^{2})(\sum _{i\in I_{k}} c_{i}^{2}) .
\end{aligned}
\end{equation*}
Summing the above over $k$ yields
\begin{equation}
\begin{aligned}
 & \sum _{k=1}^{K}\bigl[(\sum _{i\in I_{k}} a_{i} x_{i})^{2} +(\sum _{i\in I_{k}} b_{i} y_{i})^{2}\bigr]\\
\leqslant  & \sum _{k=1}^{K}\bigl[(\sum _{i\in I_{k}} h_{i}^{2})(\sum _{j\in I_{k}} c_{j}^{2})\bigr] =\sum _{k=1}^{K}\bigl[\sum _{j\in I_{k}}(\sum _{i\in I_{k}} h_{i}^{2}) c_{j}^{2}\bigr]\\
= & \sum _{k\in I_{K}}( c_{k}^{2}(\sum _{j=k}^{K}\sum _{i\in I_{j}} h_{i}^{2})) \leqslant \sum _{k\in I_{K}}( c_{k}^{2}(\sum _{j=1}^{K}\sum _{i\in I_{j}} h_{i}^{2}))\\
= & (\sum _{j=1}^{K}\sum _{i\in I_{j}} h_{i}^{2})(\sum _{k\in I_{K}} c_{k}^{2})
\end{aligned}
\end{equation}
\end{proof}

By \eqref{eq:alpha_k_beta_k} and \eqref{eq:alpha_k_beta_k_app}, 
\begin{equation}
\label{eq:delta_a_b}
\begin{aligned}
\Delta \alpha _{k} & =\hat{s}\left| \sum\nolimits _{j\in \overline{D}_{k}} t_{j}^{x,y}\left[\left( t_{j}^{y} -t_{j-1}^{x}\right)^{+} -\left( t_{j}^{y} -\mu _{j}^{x}\right)^{+}\right]\right| \\
\Delta \beta _{k} & =\hat{f}\left| \sum\nolimits _{j\in \overline{D}_{k}} t_{j}^{x,y}\left[\left( t_{j-1}^{x} -t_{j}^{y}\right)^{+} -\left( \mu _{j}^{x} -t_{j}^{y}\right)^{+}\right]\right| 
\end{aligned} ,
\end{equation}
 where we omit the subscript '$^{A}$' since no confusion will be caused. We can apply Lemma \ref{lmm:inequality_abc} to \eqref{eq:delta_a_b} by setting 
\begin{equation*}
\begin{aligned}
x_{j} & =\left( t_{j}^{y} -t_{j-1}^{x}\right)^{+} -\left( t_{j}^{y} -\mu _{j-1}^{x}\right)^{+}\\
y_{j} & =\left( t_{j-1}^{x} -t_{j}^{y}\right)^{+} -\left( \mu _{j-1}^{x} -t_{j}^{y}\right)^{+}\\
a_{j} & =\hat{s} t_{j}^{x,y}\\
b_{j} & =\hat{f} t_{j}^{x,y}\\
c_{j} & =\left| t_{j-1}^{x} -\mu _{j-1}^{x}\right| \\
h_{j} & =\max\left\{\hat{s} t_{j}^{x,y} ,\hat{f} t_{j}^{x,y}\right\}\\
I_{j} & =\overline{D}_{j}
\end{aligned} .
\end{equation*}
It's easy to verify the variables above satisfy the condition in Lemma \ref{lmm:inequality_abc}. Thus, we obtain
\begin{equation*}
\sum _{k=1}^{K} \| \Delta \mathbf{x}_{k} \| _{2}^{2} \leqslant \bigl(\sum _{j=1}^{K}\sum _{i\in \overline{D}_{j}} h_{i}^{2}\bigr)\bigl(\sum _{k\in \overline{D}_{K}}\left| t_{k-1}^{x} -\mu _{k-1}^{x}\right| ^{2}\bigr) .
\end{equation*}
Thus, for any $\epsilon < 0$,
\begin{equation*}
\begin{aligned}
 & \Pr\bigl(\sum _{k=1}^{K} \| \Delta \mathbf{x}_{k} \| _{2}^{2}  >\epsilon \bigr)\\
\leqslant  & \Pr\bigl(\bigl(\sum _{j=1}^{K}\sum _{i\in \overline{D}_{j}} h_{i}^{2}\bigr)\bigl(\sum _{k\in \overline{D}_{K}}\left| t_{k-1}^{x} -\mu _{k-1}^{x}\right| ^{2}\bigr)  >\epsilon \bigr)\\
\leqslant  & \frac{1}{\epsilon }\bigl(\sum _{j=1}^{K}\sum _{i\in \overline{D}_{j}} h_{i}^{2}\bigr)\mathbb{E}\Bigl[\sum _{k\in \overline{D}_{K}}\left| t_{k-1}^{x} -\mu _{k-1}^{x}\right| ^{2}\Bigr]\\
= & \frac{1}{\epsilon }\bigl(\sum _{j=1}^{K}\sum _{i\in \overline{D}_{j}} h_{i}^{2}\bigr)\sum _{k\in \overline{D}_{K}}\operatorname{Var}( t_{k-1})\\
= & \frac{1}{\epsilon }\bigl(\sum _{j=1}^{K}\sum _{i\in \overline{D}_{j}} h_{i}^{2}\bigr)\sum _{k\in \overline{D}_{K}}\frac{\alpha _{k-1} \beta _{k-1}}{(\alpha _{k-1} +\beta _{k-1} )^{2} (\alpha _{k-1} +\beta _{k-1} +1)}\\
<  & \frac{1}{\epsilon }\bigl(\sum _{j=1}^{K}\sum _{i\in \overline{D}_{j}} h_{i}^{2}\bigr)\sum _{k\in \overline{D}_{K}}\frac{\alpha _{k-1} \beta _{k-1}}{(\alpha _{k-1} +\beta _{k-1} )^{3}} ,
\end{aligned}
\end{equation*}
where the second inequality comes from the Markov's inequality.
